# Supplementary material for: Online Evolutionary Batch Size Orchestration for Scheduling Deep Learning Workloads in GPU Clusters
Source: arXiv:2108.03645 source file (2021-08-08)
Supplement: Supplementary file 1 [file appendix.tex]

\section{Appendix: Artifact Description/Artifact Evaluation}

\subsection{Summary of the experiments reported}
We implemented our experimental scheduling system in Python codes.
The system consists of a central controller and managers that are distributed on each node as follows.
\begin{itemize}
    \item Central controller: the controller accepts job submissions and runs the scheduler to make scheduling decisions.
    The information of each job is also stored at the controller.
    \item Distributed managers: the managers execute workers on the GPU devices and are responsible for information exchange between workers and the controller.
    The managers also continuously collect training logs and provide the information to the controller.
\end{itemize}
The components communicate with each other by remote calls of the RPyC library \cite{rpyc}.

ONES can be deployed as an independent resource manager for GPU resources, or on the top of common cluster resource manager such as Kubernetes \cite{k8s} with GPU support.
The scheduler exposes an API for users to submit jobs with training scripts, initial batch sizes and corresponding learning rates.
% Then it continuously optimizes the scheduling solution and deploys the optimal schedule on the GPUs in the shared cluster.
When deployed on the top of some cluster resource manager such as Kubernetes, the scheduler acts as an broker between users and the resource manager by determining resource allocation and then running each worker of the jobs on a specified GPU.

\begin{figure}[t]
    \centering
    \begin{subfigure}[t]{0.48\linewidth}
        \centering
        \includegraphics[width=\linewidth]{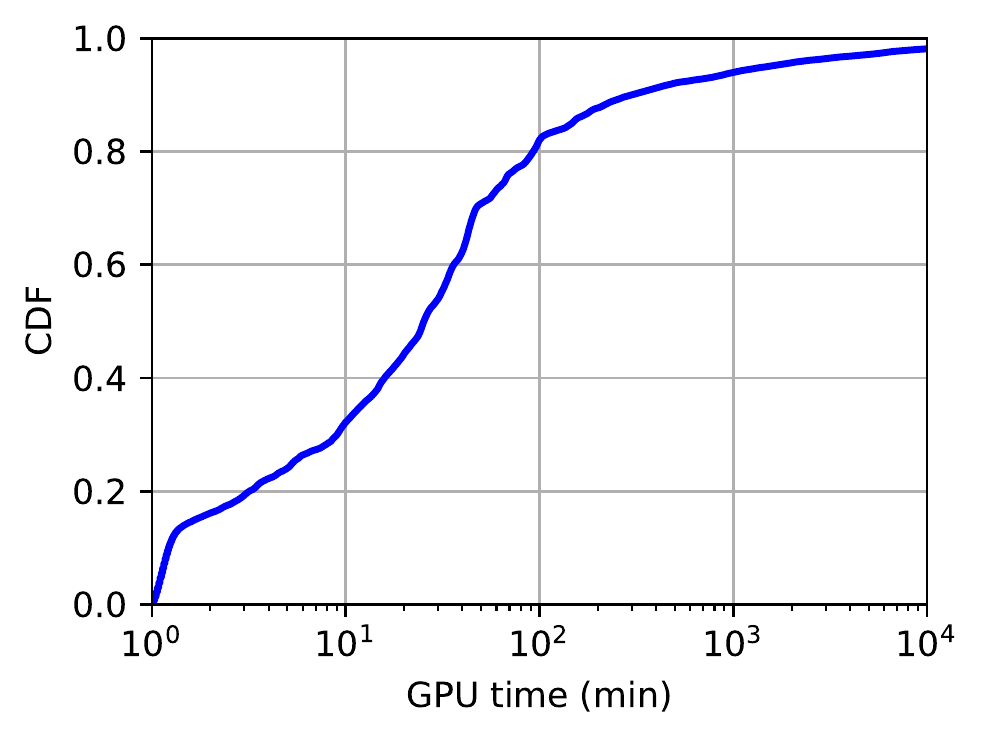}
        \caption{Microsoft traces}
    \end{subfigure}
    \begin{subfigure}[t]{0.48\linewidth}
        \centering
        \includegraphics[width=\linewidth]{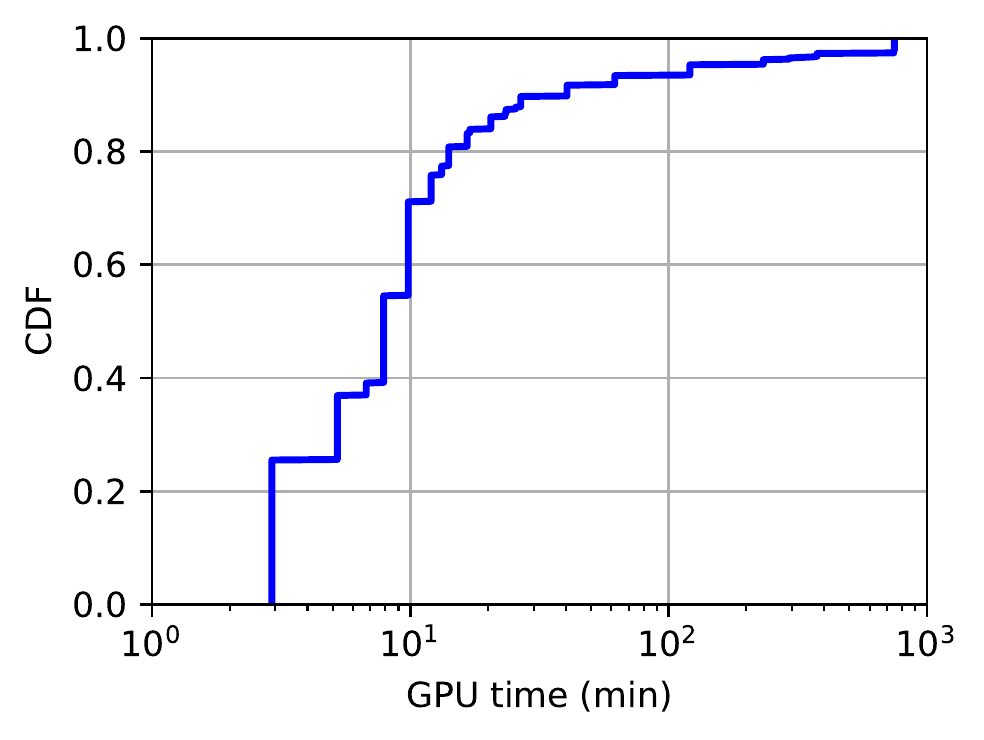}
        \caption{Custom trace}
    \end{subfigure}
    \caption{Comparison between GPU time distributions of jobs in  real trace and our custom trace.}
    \label{fig:trace}
\end{figure}

In our experiments, we used our custom job traces that were generated by simulating the characteristics of the public production traces from Microsoft \cite{jeon2019analysis}.
To generate a similar GPU utilization (\#GPUs $\times$ execution time) distribution to the Microsoft traces, we uniformly sampled 400 jobs from the Microsoft traces and replace each with a job in \autoref{tab:jobs} that has the closest GPU time.
The GPU time distribution of our custom trace is illustrated in \autoref{fig:trace}, compared with the Microsoft traces.
Besides, job arrivals follow a Poisson process, where its average arrival time interval and the average job length has the same ratio as those in the Microsoft traces.

We implemented the jobs in Pytorch, with very few lines of changes in common training codes to enable the elastic batch size scaling.
Some example codes are shown in \autoref{alg:scaling}.
With the \texttt{distributed} package, in line 3-4, the user needs to create a scaling agent with the corresponding IP address and port of the worker, then load the job execution information such as the model, optimizer, loss function and dataset into the scaling agent.
Then in line 13-15 in the training loop, the user needs to check \texttt{sa.scaling\_flag} and call \texttt{sa.scale()}.
The method will invoke the scaling agent to automatically communicate with the central scheduler to execute batch size scaling in background, as described in \S \ref{sec:orchest}.

\lstset{
captionpos=b,
basicstyle=\ttfamily\small,
numbers=left,
numberstyle=\small,
frame = single,
language=Python,
tabsize=4}

\begin{lstlisting}[caption={Example codes of enabling batch size scaling with ONES in PyTorch}, label=alg:scaling, float, floatplacement=t]
import distributed

sa = distributed.ScalingAgent(ip_addr, port)
model, optimizer, loss_fn, dataloader = \
    sa.load(user_model, user_optimizer,
            user_loss_fn, user_dataset)

while not converge:
    for inputs, targets in dataloader:
    	### forward & backward
    	...
    	###
    	if sa.scaling_flag:
    		model, dataloader = sa.scale()
    		break
\end{lstlisting}

\subsection{Artifact availability}
\textit{Software Artifact Availability:}
Some author-created software artifacts are NOT maintained in a public repository or are NOT available under an OSI-approved license.

\textit{Hardware Artifact Availability:}
There are no author-created hardware artifacts.

\textit{Data Artifact Availability:}
Some author-created data artifacts are NOT maintained in a public repository or are NOT available under an OSI-approved license.

\textit{Proprietary Artifacts:}
No author-created artifacts are proprietary.

\textit{List of URLs and/or DOIs where artifacts are available:}
Not published; Available upon request.

\subsection{Baseline experiments setup, and modifications made for the paper}
\textit{Relevant hardware details:}
We ran all the experiments on a platform of 4 GPU servers. Each server has Xeon W-2133 CPU, 64GBmemory and 4 NVIDIA RTX2080Ti GPUs.

\textit{Operating systems and versions:}
All experiments were run on Ubuntu 18.04 LTS.

\textit{Compilers and versions:}
Python v3.6

\textit{Libraries and versions:}
Pytorch v1.0.1, CUDA v10.1, cuDNN v7.6.5, RPyC v5.0.1.

\textit{Paper Modifications:}
We implemented the baseline scheduling algorithms in Python and added them into the controller.

\subsection{Artifact evaluation}
\textit{Verification and validation studies:}
We used the same job traces to validate ONES with the baselines.
The traces include typical DL models and datasets that are popularly used in the experiments of baseline papers.

\textit{Accuracy and precision of timings:}
Each behavior of the jobs, including job submission, start, pausing, resuming, and completion, was printed in logs at real time.
We collected the experimental results from the logs to present the performance evaluations.

\textit{Used manufactured solutions or spectral properties:}
Not applicable.

\textit{Quantified the sensitivity of results to initial conditions and/or parameters of the computational environment:}
We used the same settings with the baseline.

\textit{Controls, statistics, or other steps taken to make the measurements and analyses robust to variability and unknowns in the system:}
We ran all the experiments for three times and take the average over the results.
